# Supplementary material for: LITE: A Paradigm Shift in Multi-Object Tracking with Efficient ReID Feature Integration
Source: arXiv:2409.04187 source file (2024-10-01)
Supplement: Supplementary file 1 [file 6390-supplementary.pdf]

# LITE: A Paradigm Shift in Multi-Object Tracking with Efficient ReID Feature Integration


Jumabek Alikhanov[1[0000−0003−3103−6033]], Dilshod Obidov[1[0009−0007−9845−6979]] and Hakil Kim[1[0000−0003−4232−3804]]

Department of Electrical and Computer Engineering, Inha University, Incheon 402-751, South Korea
`juma@inha.edu`, `dilshod@humblebee.ai`, `hikim@inha.ac.kr`
*Corresponding author: Hakil Kim (e-mail: hikim@inha.ac.kr)*


## 1 Proposed Evaluation Framework

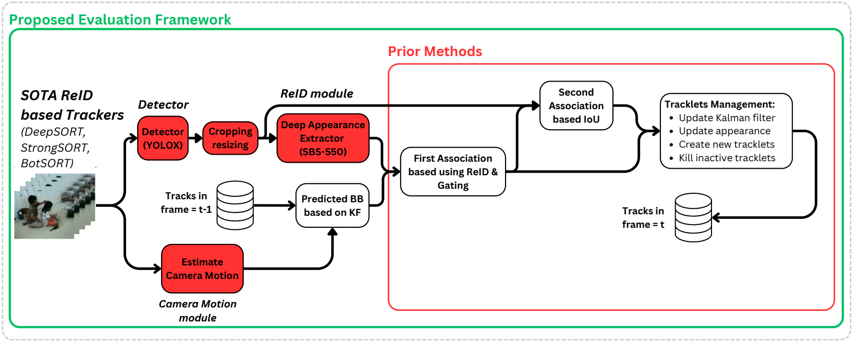


**Fig. 1:** Holistic Evaluation Framework: Red shows current MOT evaluation methodologies. Green for proposed framework.

## 2 Qualitative Results

**Fig. 2:** Comparative Analysis of Tracking Methods on MOT17-04-FRCNN

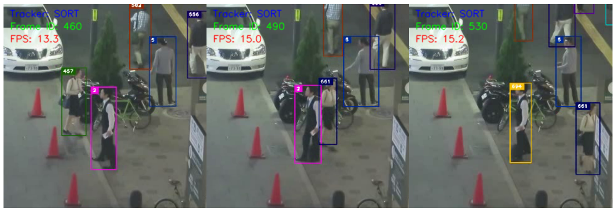

**(a)** Frame 460 **(b)** Frame 490 **(c)** Frame 530

SORT: ID switches after path crossing, showing the need for appearance features

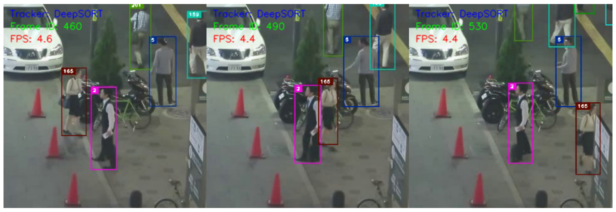

**(d)** Frame 460 **(e)** Frame 490 **(f)** Frame 530

DeepSORT: Path crossing situation handled without ID switches

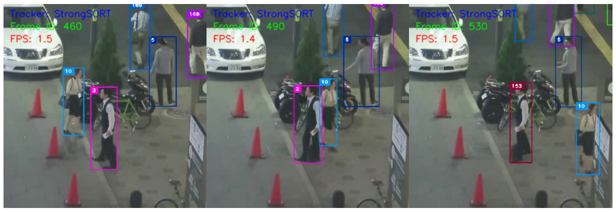

**(g)** Frame 460 **(h)** Frame 490 **(i)** Frame 530

StrongSORT: ID switch noted once object had in place movements

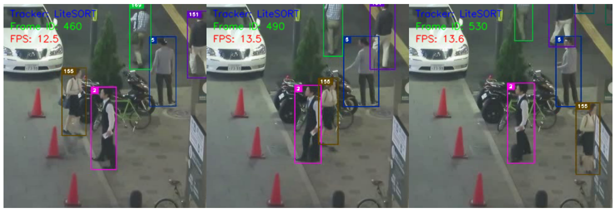

**(j)** Frame 460 **(k)** Frame 490 **(l)** Frame 530

LiteSORT: No ID switches after path crossing

Comparative Analysis of Tracking Methods on MOT20-01

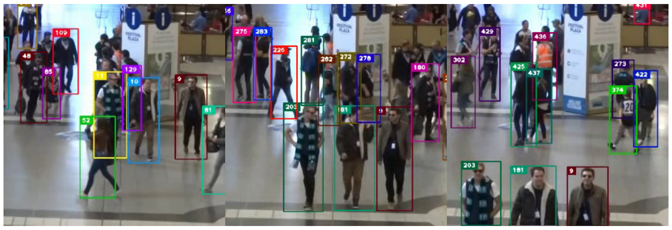

**(a)** Frame 100 **(b)** Frame 200 **(c)** Frame 300

SORT: ID switches occurred between frames 100 and 200

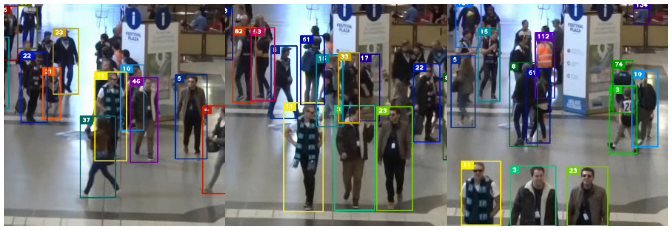

**(d)** Frame 100 **(e)** Frame 200 **(f)** Frame 300

DeepSORT: Few ID switches noted from frame 100 to 200

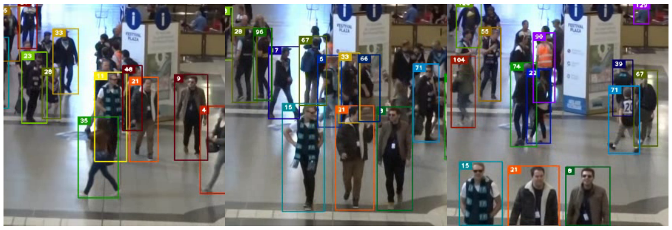

**(g)** Frame 100 **(h)** Frame 200 **(i)** Frame 300

StrongSORT: Managed tracking with few ID switches

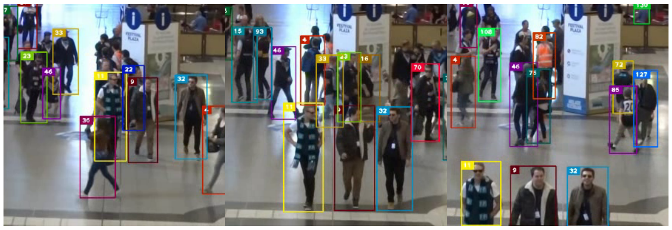

**(j)** Frame 100 **(k)** Frame 200 **(l)** Frame 300

LiteSORT: Consistently tracked without ID switches

**Fig. 3:** In this scenario, three men walking from the center of the frame are tracked from frame 100 to frame 300. The sequence tests each tracker's ability to maintain consistent identification amidst movement and occlusions.

Comparative Analysis of Tracking Methods on MOT17-09-FRCNN

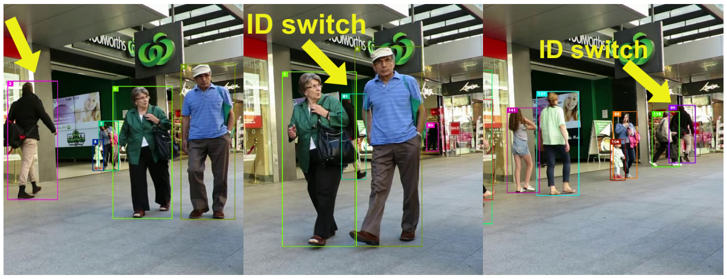


**(a)** Frame 90 **(b)** Frame 130 **(c)** Frame 225

SORT: ID switches noted, showing the need for appearance features

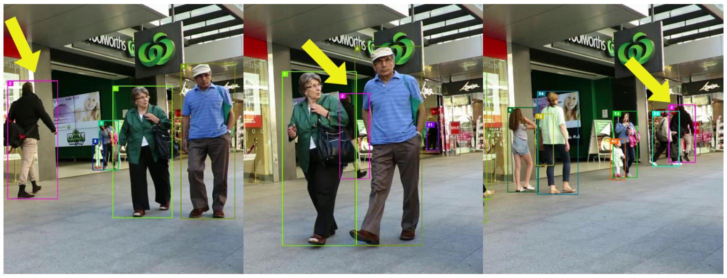

**(d)** Frame 90 **(e)** Frame 130 **(f)** Frame 225

DeepSORT: Tracked target object

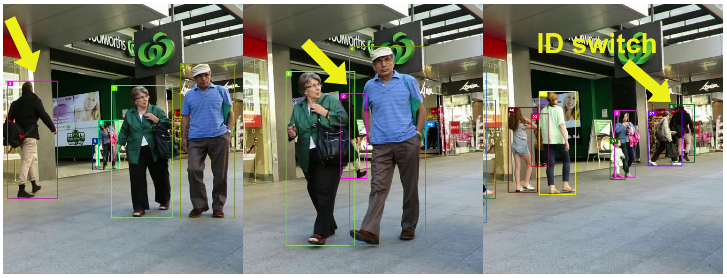


**(g)** Frame 90 **(h)** Frame 130 **(i)** Frame 225

StrongSORT: ID switch noted

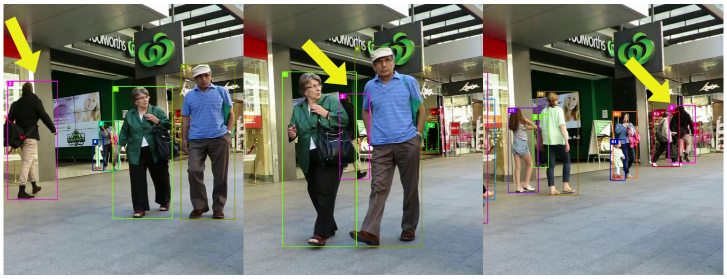

**(j)** Frame 90 **(k)** Frame 130 **(l)** Frame 225

LiteSORT: Tracked target object

**Fig. 4:** In this scenario, a person in a black hoodie is taken as the target. The individual moves from the left side to the right side of the frame while other objects occasionally block the view, causing occlusions. These occlusions challenge the trackers' ability to maintain consistent tracking of the target, leading to varying levels of performance among different tracking methods.

Comparative Analysis of Tracking Methods on MOT17-10-FRCNN

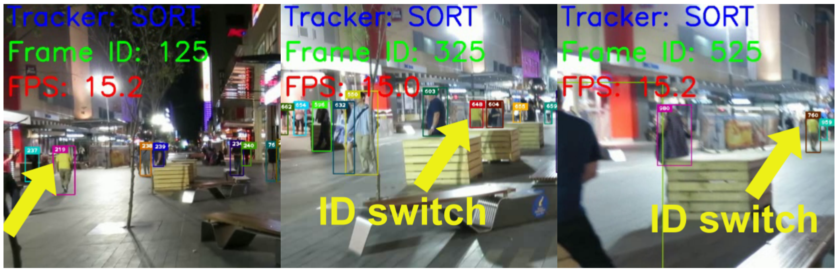


**(a)** Frame 125 **(b)** Frame 325 **(c)** Frame 525

SORT: ID switches noted, showing the need for appearance features

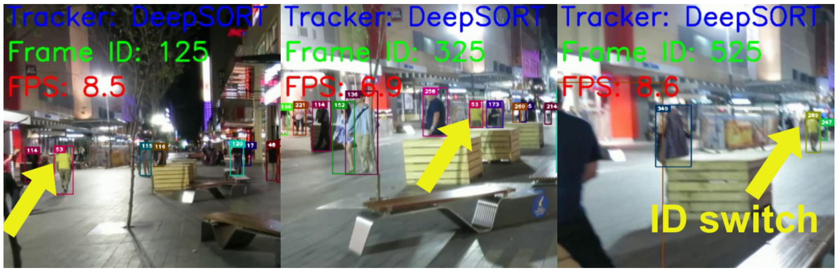


**(d)** Frame 125 **(e)** Frame 325 **(f)** Frame 525

DeepSORT: ID switch occurred

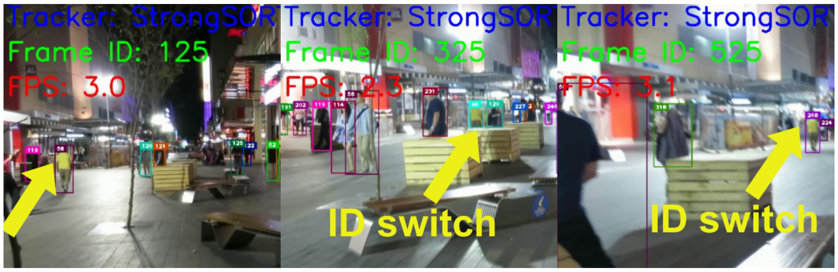


**(g)** Frame 125 **(h)** Frame 325 **(i)** Frame 525

StrongSORT: ID switches noted

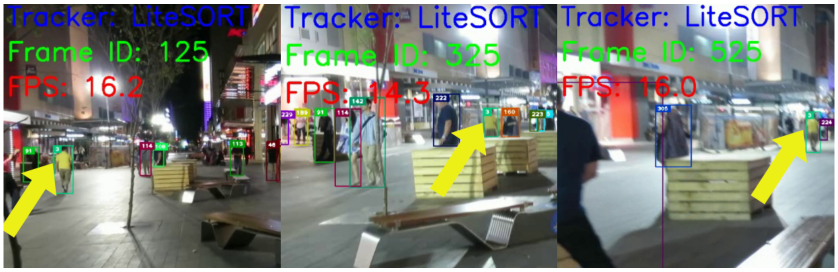


**(j)** Frame 125 **(k)** Frame 325 **(l)** Frame 525

LiteSORT: Tracked target object

**Fig. 5:** In this scenario, the target is a person in a yellow T-shirt being tracked from frame 125 to frame 525. Significant occlusions caused by other objects passing by present a challenge for the trackers to maintain accurate identification and tracking. This sequence tests the robustness of each tracking algorithm in handling occlusions and maintaining consistent target identification.

Comparative Analysis of Tracking Methods on PersonPath22 uid-vid-00096

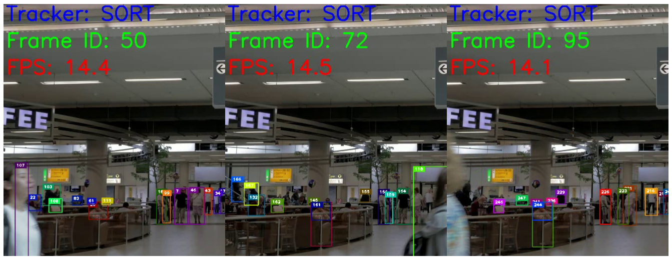


**(a)** Frame 50 **(b)** Frame 72 **(c)** Frame 95

SORT: During occlusions, frequent ID switches occur.

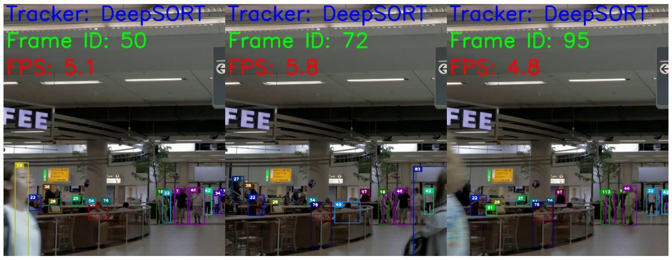


**(d)** Frame 50 **(e)** Frame 72 **(f)** Frame 95

DeepSORT: Maintains good ID consistency despite occlusions.

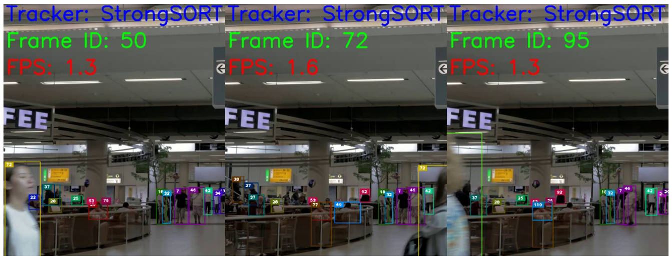


**(g)** Frame 50 **(h)** Frame 72 **(i)** Frame 95

StrongSORT: Handles occlusions well with some ID switches

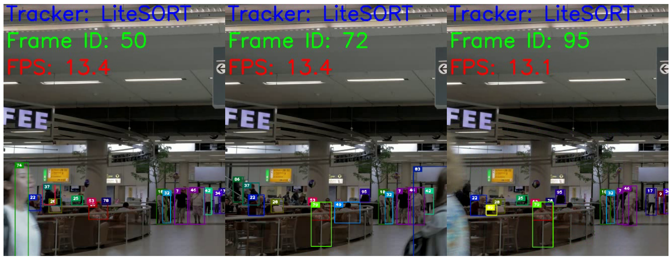


**(j)** Frame 50 **(k)** Frame 72 **(l)** Frame 95

LiteSORT: Manages occlusions with few ID switches.

**Fig. 6:** In this scenario, from frame 50 to frame 72, a person passes near the camera, blocking the view and occluding other objects. This occlusion causes challenges for the trackers in maintaining accurate tracking of the occluded objects. The issue continues from frame 72 to frame 95, where another person passes by the camera, causing further occlusions. These occlusions lead to ID switches and tracking errors, demonstrating the varying robustness of different trackers.

Comparative Analysis of Tracking Methods on PersonPath22 uid-vid-00030

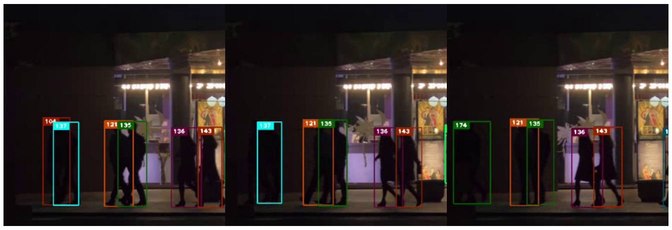

**(a)** Frame 180 **(b)** Frame 195 **(c)** Frame 210

SORT: Maintains consistent tracking due to its focus on motion rather than appearance features.

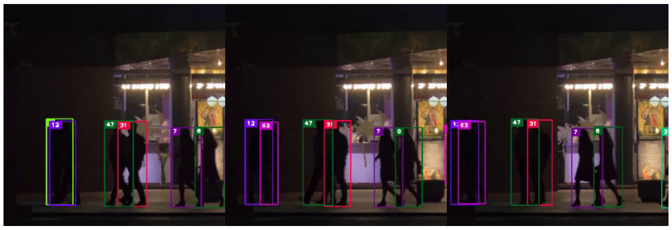

**(d)** Frame 180 **(e)** Frame 195 **(f)** Frame 210

DeepSORT: Struggles with low-light, leading to tracking errors and ID switches.

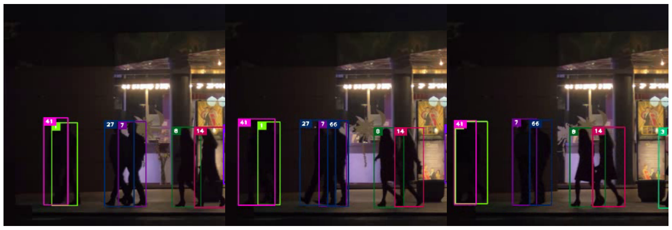

**(g)** Frame 180 **(h)** Frame 195 **(i)** Frame 210

StrongSORT: Performs relatively well, but still faces some challenges in low-light conditions.

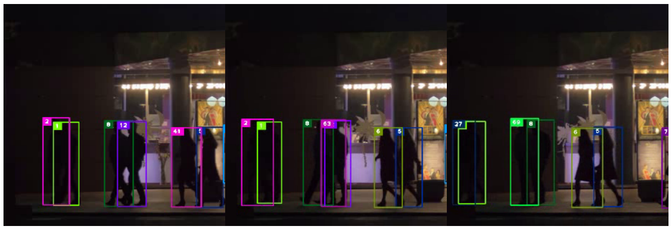

**(j)** Frame 180 **(k)** Frame 195 **(l)** Frame 210

LiteSORT: Encounters challenges in low-light, resulting in tracking inaccuracies and ID switches.

**Fig. 7:** In this scenario, all trackers are tested under challenging low-light conditions. The dark environment presents difficulties in maintaining accurate tracking, especially for trackers relying on appearance features. Despite these challenges, SORT performs noticeably better than the others, as its tracking method is less dependent on appearance features and more focused on motion, which remains relatively consistent even in low-light conditions.

# 3 Discussion

## 3.1 Analysis of the Experimental Results

The proposed evaluation framework paves the way for future research for deeper investigation of tracking pipelines components. For instance, matching thresholds of trackers, tentative period before confirming a track, and track elimination expiration threshold can be analyzed more deeply. It is also noteworthy to mention detector settings such as whether quantization is used, NMS thresholds.

## 3.2 Strengths and Limitations

The simple yet profound contribution of LITE paradigm is to obtain ReID features without extra computation. We showed its usefulness by applying this paradigm to simple tracker DeepSORT which resulted in a tracker named LiteSORT. Results show that LiteSORT keeps the same HOTA score as DeepSORT while improving the speed two times. While LiteSORT has the advantage of being fast, we believe there can be more work done to increase its accuracy (i.e., HOTA score) by further engineering on how to exploit activation features extracted from pre-trained detectors directly.

Further, LITE paradigm can be applied to other ReID based trackers in the same fashion. However, this is the outside of scope of this work.
